# Supplementary material for: MolDeTox: Evaluating Language Model's Stepwise Fragment Editing for Molecular Detoxification
Source: arXiv:2605.12181 source file (2026-05-12)
Supplement: Supplementary file 1 [file main_step_wise_analysis.tex]

\section{Step-wise Success Dependency Analysis}

\input{Tables/Appendix_step_success_case_def}

To better understand how models reach final success or failure, we group each aligned test sample into one of eight outcome cases defined by the correctness pattern of Task~1, Task~2, and Task~3. Table~\ref{tab:stepwise_case_definition} defines these cases, and Table~\ref{tab:stepwise_final_composition} summarizes how they are distributed within the final success ($T3=1$) and final failure ($T3=0$) groups.

A first observation from Table~\ref{tab:stepwise_final_composition} is that final failures are dominated by C000 (Complete Failure). The pooled Overall proportion of C000 within the $T3=0$ group is 0.7695, far larger than any other failure-side case. This indicates that most failed Task~3 samples are not near-miss outcomes, but rather correspond to collapse across all three tasks.

At the same time, failure is not exclusively driven by total collapse. The second-largest failure-side component is C100 (Identification-only Success), with an Overall proportion of 0.1956. This suggests that a meaningful subset of failed samples already identifies the toxic fragment correctly, but does not carry that partial progress through to successful replacement and final molecule generation.

The success-side composition shows a different pattern. In Table~\ref{tab:stepwise_final_composition}, successful samples are concentrated on C111 (Complete Success) and C101 (Identification-led Success), with Overall proportions of 0.4297 and 0.3133, respectively. Thus, final success most often arises either from fully correct step-wise reasoning or from cases in which the toxic-fragment identification stage is already strong enough to support the final output.

The model-wise breakdown further shows that stronger in-context prompting changes the internal structure of success. Among successful GPT-5.2 samples, the share of C111 increases from 0.3158 to 0.5379 under 4-shot prompting, while for Qwen3-4B it rises from 0.0000 to 0.3077. This suggests that 4-shot prompting does not merely increase the number of successful outputs, but shifts successful behavior toward more fully coherent step-wise success patterns. The Qwen3-4B success-side distribution should be interpreted cautiously, however, since its base model has only one successful sample.

Taken together, these results show that the benchmark captures more than final correctness alone. Table~\ref{tab:stepwise_case_definition} provides the semantic meaning of each case, and Table~\ref{tab:stepwise_final_composition} reveals how final success and failure are internally composed. The resulting picture is that most failures arise from complete breakdown, whereas successful detoxification is concentrated in cases with strong or fully correct intermediate reasoning, and stronger prompting shifts the distribution further toward complete success.
